# Supplementary material for: Neutrino masses and mixings in the baryon triality constrained minimal supersymmetric standard model
Source: arXiv:1106.4338 source file (2011-06-21)
Supplement: Supplementary file 1 [file appendix.tex]

\begin{appendix}

\section{$\chi^2$ definition}
\label{appendix:chi2}
We minimize the following $\chi^2$
with \minuit:
\bit
\item normal hiearchy:
\begin{align}
4\chi^2_{NH} =&\left(\frac{\Delta m^2_{21}-7.59\times10^{-5}} {
   0.2\times10^{-5}}\right)^2+ 
  \left( \frac{\Delta m^2_{31} - 2.45\times10^{-3}} { 0.1\times10^{-3}}\right)^2 + \nonumber \\
 &\left(\frac{\sin^2(\theta_{12})  - 0.31}{ 0.02}\right)^2 +  \left(\frac{\sin^2(\theta_{23})  -
  0.51}{0.06}\right)^2.
\end{align}
\item inverted hierarchy:
\begin{align}
4\chi^2_{IH} =&\left(\frac{\Delta m^2_{21}-7.59\times10^{-5}} {
   0.2\times10^{-5}}\right)^2+ 
  \left( \frac{\Delta m^2_{31}+2.34\times10^{-3}} { 0.1\times10^{-3}}\right)^2 + \nonumber \\
 &\left(\frac{\sin^2(\theta_{12})  - 0.31}{ 0.02}\right)^2 +  \left(\frac{\sin^2(\theta_{23})  -
  0.51}{0.06}\right)^2.
 \end{align}
\eit

\section{Old Tables}
\begin{widetext}

\begin{table}[h!]
\begin{tabular}{|c|c|c|c|c|c|c|c|c|c|} 
\hline
& & $l_1$ & $l_2$ & $l_3$ & $l_1^\prime$ & $l_2^\prime$ & $l_3^\prime$ & $m_{\rm{LSP}}$ [GeV]\\
\hline
\hline
NH1a & BP1a &  & $0.145$ & $0.166$ &  $ 2.46 \cdot 10^{-4}$ & $3.32\cdot10^{-4}$ & $-1.81\cdot10^{-4}$ & $191.88\,(\tilde e)$\\
& up & & $\lam_{211}$ & $\lam_{311}$ & $\lamp_{111}$ & $\lamp_{211}$ & $\lamp_{311}$&\\
\hline
NH1a & BP1a &  & $0.153$ & $0.159$ &  $ 2.45 \cdot 10^{-4}$ & $-2.10\cdot10^{-4}$ & $3.13 \cdot10^{-4}$ & $191.92\,(\tilde \tau)$\\
sign & up & & $\lam_{211}$ & $\lam_{311}$ & $\lamp_{111}$ & $\lamp_{211}$ & $\lamp_{311}$&\\
\hline
NH1a & BP1a &  & $0.154$ & $0.159$ &  $ 1.20 \cdot 10^{-4}$ & $-1.02\cdot10^{-4}$ & $1.52 \cdot10^{-4}$ & $191.92\,(\tilde \tau)$\\
sign & down & & $\lam_{211}$ & $\lam_{311}$ & $\lamp_{111}$ & $\lamp_{211}$ & $\lamp_{311}$&\\
\hline
NH1b & BP1a &  & $0.0178$ & $0.0182$ &  $ -0.0090$ & $-0.0296$ & $0.0182$ & $162.46\,(\tilde \tau$)\\
& up & & $\lam_{211}$ & $\lam_{311}$ & $\lamp_{111}$ & $\lamp_{211}$ & $\lamp_{311}$&\\
\hline
NH1b & BP1a &  & $0.01477$ & $0.01479$ &  $ -0.00545 $ & $-0.00894$ & $-0.0210$ & $162.46\,(\tilde \tau$)\\
& down & & $\lam_{211}$ & $\lam_{311}$ & $\lamp_{111}$ & $\lamp_{211}$ & $\lamp_{311}$&\\
\hline
NH1a & BP3old &  & $0.148$ & $0.0168$ &  $ 2.61\cdot10^{-4}$ & $3.50\cdot10^{-4}$ & $-1.96\cdot10^{-4}$ & $136.4\,(\tilde e)$\\
& up & & $\lam_{211}$ & $\lam_{311}$ & $\lamp_{111}$ & $\lamp_{211}$ & $\lamp_{311}$&\\
\hline
\mtext{ NH1a} & BP1b & & $0.177$ &$ 0.201 $& $ 3.27 \cdot 10^{-4}$ & $ 3.69 \cdot 10^{-4}$ & $ -3.09 \cdot 10^{-4}$ &$294.9\,(\chi_0)$\\
& up & & $\lam_{211}$ & $\lam_{311}$ & $\lamp_{111}$ & $\lamp_{211}$ & $\lamp_{311}$&\\ %chi2=0.04 good!
\hline
\mtext{ NH1b} & BP1b & & $0.014$ &$ 0.014 $&$ 0.010 $ & $ 0.010 $ & $- 0.009 $ &$293.5\,(\chi_0)$\\
& up & & $\lam_{211}$ & $\lam_{311}$ & $\lamp_{111}$ & $\lamp_{211}$ & $\lamp_{311}$&\\ %chi2=0.2 
\hline
\hline
NH3a & BP1a & $ 1.38\cdot10^{-5}$& $2.7\cdot10^{-5}$ & $   $ &  $ -8.64\cdot10^{-8}$ & $7.55\cdot10^{-7}$ & $9.93\cdot10^{-7}$ & $192.4\,(\tilde \tau)$\\
& up& $\lam_{133}$& $\lam_{233}$ &  & $\lamp_{133}$ & $\lamp_{233}$ & $\lamp_{333}$&\\
\hline
NH3b & BP1a & $ 1.4\cdot10^{-6}$& $2.6\cdot10^{-6}$ & $   $ &  $ -3.2\cdot10^{-6}$ & $3.5\cdot10^{-5}$ & $4.1\cdot10^{-5}$ & $163.4\,(\tilde \tau)$\\
& up& $\lam_{133}$& $\lam_{233}$ &  & $\lamp_{133}$ & $\lamp_{233}$ &
$\lamp_{333}$&\\
\hline
\hline
\mtext{NH3a} & BP1b & $ -2.01\cdot10^{-5}$& $-4.32\cdot10^{-5}$ & $   $ &  $
-6.66\cdot10^{-8}$ & $-1.15\cdot10^{-6}$ & $-1.09\cdot10^{-6}$ &
$294.9\,(\chi_0)$\\ %bad convergence!! chi2=0.46!!, sintheta23^2=0.4
& up& $\lam_{133}$& $\lam_{233}$ &  & $\lamp_{133}$ & $\lamp_{233}$ &
$\lamp_{333}$&\\
\hline
NH3a & BP2 (Higgs!!) & $ 1.3\cdot10^{-5}$& $2.4\cdot10^{-5}$ & $   $ & % higgs not violated if we increase tanb to e.g. 25!
$ 1.1 \cdot10^{-7}$ & $-4.4\cdot10^{-7}$ & $-8.6\cdot10^{-7}$ & $109.2\,(\tilde \tau)$\\
& up& $\lam_{133}$& $\lam_{233}$ &  & $\lamp_{133}$ & $\lamp_{233}$ & $\lamp_{333}$&\\
\hline
NH3a & BP3 & $ 5.8\cdot10^{-5}$& $1.1\cdot10^{-4}$ & $   $ &
$ -5.4 \cdot10^{-7}$ & $9.6\cdot10^{-6}$ & $1.2\cdot10^{-5}$ & $142.0\,(\chi_0)$\\
& up& $\lam_{133}$& $\lam_{233}$ &  & $\lamp_{133}$ & $\lamp_{233}$ &
$\lamp_{333}$&\\
\hline
NH3a & BP2 (Higgs!!) & $ 1.2\cdot10^{-5}$& $2.6\cdot10^{-5}$ & $   $ &
% a0=117.8
$ -1.2 \cdot10^{-7}$ & $1.1\cdot10^{-6}$ & $1.1\cdot10^{-6}$ & $109.2\,(\tilde \tau)$\\
& up, sgn-!& $\lam_{133}$& $\lam_{233}$ &  & $\lamp_{133}$ & $\lamp_{233}$ & $\lamp_{333}$&\\
\hline
NH3a & BP3 & $ 5.0\cdot10^{-5}$& $1.1\cdot10^{-4}$ & $   $ &
% A0=-147.5 due to high m0, sgnmu!
$ -1.1 \cdot10^{-6}$ & $1.2\cdot10^{-5}$ & $1.2\cdot10^{-6}$ & $144.9\,(\chi_0)$\\
& up, sgn-!& $\lam_{133}$& $\lam_{233}$ &  & $\lamp_{133}$ & $\lamp_{233}$ & $\lamp_{333}$&\\
\hline
\end{tabular}
\caption{Best fit points for normal hierarchy.}
\label{tab:NH}
\end{table}

\begin{table}[h!]
\scriptsize\begin{tabular}{|c|c|c|c|c|c|c|c|c|c|c|c|c|} 
\hline

& & $l_1$ & $l_2$ & $l_3$ & $l_4$ & $l_5$ & $l_6$ & $l_1^\prime$ & $l_2^\prime$ & $l_3^\prime$ & $m_{\rm{LSP}}$ [GeV]\\
\hline
\hline
DEG1 & BC1b & $-7.29\cdot10^{-6}$ & $6.83\cdot10^{-6}$ & $-9.46\cdot10^{-6}$ & $-0.283$ & $-4.87\cdot10^{-5}$ & $4.39\cdot10^{4}$ & $-8.49\cdot10^{-5}$ & $3.54\cdot10^{-5}$ & $-6.45\cdot10^{-5}$& \\
NH& up & $\lam_{133}$ & $\lam_{233}$ & $\lam_{322}$ & $\lam_{231}$ & $\lam_{213}$ & $\lam_{312}$ & $\lamp_{133}$ & $\lamp_{233}$ & $\lamp_{333}$&\\
\hline
DEG1 & BC1b & $8.41\cdot10^{-6}$ & $5.07\cdot10^{-6}$ & $-8.69\cdot10^{-6}$ & $-0.302$ & $-2.88\cdot10^{-5}$ & $4.01\cdot10^{4}$ & $-8.68\cdot10^{-5}$ & $3.94\cdot10^{-5}$ & $-6.20\cdot10^{-5}$& \\
NH& down & $\lam_{133}$ & $\lam_{233}$ & $\lam_{322}$ & $\lam_{231}$ & $\lam_{213}$ & $\lam_{312}$ & $\lamp_{133}$ & $\lamp_{233}$ & $\lamp_{333}$&\\
\hline
DEG2 & BC1b & $9.72\cdot10^{-6}$ & $-3.86\cdot10^{-6}$ & $6.03\cdot10^{-6}$ & $-0.381$ & $1.83\cdot10^{-5}$ & $-7.50\cdot10^{4}$ & $5.76\cdot10^{-5}$ & $7.03\cdot10^{-5}$ & $-5.91\cdot10^{-5}$& \\
NH& up & $\lam_{133}$ & $\lam_{233}$ & $\lam_{322}$ & $\lam_{231}$ & $\lam_{213}$ & $\lam_{312}$ & $\lamp_{133}$ & $\lamp_{233}$ & $\lamp_{333}$&\\
\hline
DEG2 & BC1b & $9.93\cdot10^{-6}$ & $-3.66\cdot10^{-6}$ & $5.87\cdot10^{-6}$ & $-0.401$ & $1.31\cdot10^{-5}$ & $-6.85\cdot10^{4}$ & $5.69\cdot10^{-5}$ & $7.37\cdot10^{-5}$ & $-5.90\cdot10^{-5}$& \\
NH& down & $\lam_{133}$ & $\lam_{233}$ & $\lam_{322}$ & $\lam_{231}$ & $\lam_{213}$ & $\lam_{312}$ & $\lamp_{133}$ & $\lamp_{233}$ & $\lamp_{333}$&\\
\hline

DEG2 & BC1b & $1.02\cdot10^{-6}$ & $-3.79\cdot10^{-6}$ & $4.84\cdot10^{-6}$ & $0.499$ & $-7.61\cdot10^{-5}$ & $-2.14\cdot10^{-4}$ & $5.03\cdot10^{-5}$ & $9.00\cdot10^{-5}$ & $-6.83\cdot10^{-5}$& \\
IH& up & $\lam_{133}$ & $\lam_{233}$ & $\lam_{322}$ & $\lam_{231}$ & $\lam_{213}$ & $\lam_{312}$ & $\lamp_{133}$ & $\lamp_{233}$ & $\lamp_{333}$&\\
\hline
DEG2 & BC1b & $9.62\cdot10^{-6}$ & $-4.24\cdot10^{-6}$ & $6.62\cdot10^{-6}$ & $0.361$ & $1.79\cdot10^{-5}$ & $-7.65\cdot10^{-4}$ & $5.62\cdot10^{-5}$ & $7.17\cdot10^{-5}$ & $-6.17\cdot10^{-5}$& \\
IH& down & $\lam_{133}$ & $\lam_{233}$ & $\lam_{322}$ & $\lam_{231}$ & $\lam_{213}$ & $\lam_{312}$ & $\lamp_{133}$ & $\lamp_{233}$ & $\lamp_{333}$&\\
\hline

DEG3 & BC1b & $9.72\cdot10^{-6}$ & $-3.86\cdot10^{-6}$ & $6.03\cdot10^{-6}$ & $-0.381$ & $1.83\cdot10^{-5}$ & $-7.50\cdot10^{4}$ & $5.76\cdot10^{-5}$ & $7.03\cdot10^{-5}$ & $-5.91\cdot10^{-5}$& \\
NH& up & $\lam_{133}$ & $\lam_{233}$ & $\lam_{322}$ & $\lam_{231}$ & $\lam_{213}$ & $\lam_{312}$ & $\lamp_{133}$ & $\lamp_{233}$ & $\lamp_{333}$&\\
\hline
\hline
& & $l_1^\prime$ & $l_2^\prime$ & $l_3^\prime$ & $l_4^\prime$ & $l_5^\prime$ & $l_6^\prime$ & $l_7^\prime$ & $l_8^\prime$ &  & $m_{\rm{LSP}}$ [GeV]\\
\hline
\hline
DEG4 & BC1b & $6.64\cdot10^{-3}$ & $-7.13\cdot10^{-3}$ & $6.70\cdot10^{-3}$ & $2.81\cdot10^{-4}$ & $3.06\cdot10^{-4}$ & $1.54\cdot10^{3}$ & $7.81\cdot10^{-4}$ & $-7.21\cdot10^{-4}$ &  &\\
NH& up& $\lamp_{112}$ & $\lamp_{212}$ & $\lamp_{312}$ & $\lamp_{232}$ & $\lamp_{332}$ & $\lamp_{131}$ & $\lamp_{231}$ & $\lamp_{331}$ &\\
\hline
\hline
& & $l_1^\prime$ & $l_2^\prime$ & $l_3^\prime$ & $l_4^\prime$ & $l_5^\prime$ & $l_6^\prime$ & $l_1$ & $l_2$ &  & $m_{\rm{LSP}}$ [GeV]\\
\hline
\hline
STEVE DEG & BC1a & $-7.93\cdot10^{-5}$ & $4.31\cdot10^{-5}$ & $-3.14\cdot10^{-5}$ & $-1.94\cdot10^{-3}$ & $-1.51\cdot10^{-3}$ & $2.83\cdot10^{-3}$ & $-3.1\cdot10^{-2}$ & $-1.80\cdot10^{-2}$ &  &\\
NH& up& $\lamp_{133}$ & $\lamp_{233}$ & $\lamp_{333}$ & $\lamp_{122}$ & $\lamp_{222}$ & $\lamp_{322}$ & $\lam_{211}$ & $\lam_{311}$ &\\
\hline
\end{tabular}
\caption{Best fit points for degenerate neutrino masses.}
\label{tab:DEG}
\end{table}

\end{widetext}

\end{appendix}
